# Supplementary material for: Polar hairs of mixed-parity nodal superconductors in Rarita-Schwinger-Weyl metals
Source: arXiv:2211.02649 ancillary file (2023-05-16)
Supplement: Supplementary file 1 [file Supplementary.pdf]

# Supplementary Materials: Polar hairs of mixed-parity nodal superconductors in Rarita-Schwinger-Weyl metals

Saswata Mandal[1] and Bitan Roy[2]

[1]*Department of Physics, Indian Institute of Science, Bangalore 560012, India*
[2]*Department of Physics, Lehigh University, Bethlehem, Pennsylvania, 18015, USA*
(Dated: November 3, 2022)

In these Supplementary Materials, we describe the band diagonalization procedure and projection of the superconducting pairings on the Fermi surface for the spin-3/2 models, encompassing both Rarita-Schwinger-Weyl (RSW) and Luttinger systems [Sec. S1]. Subsequently, we discuss the evolution of the polar hairs and nodal rings in RSW systems with pairing amplitudes [Sec. S2]. Finally, we also discuss the gap equation for the RSW systems and derive the relations between coupling strength, critical temperatures and pairing amplitudes under different conditions and show that the BCS scaling is always satisfies [Sec. S3].

## S1. BAND DIAGONALIZATION : GENERAL PROCEDURE

Here we elaborate on the band diagonalization scheme to diagonalize the Nambu-doubled Hamiltonian. Then we sought out the projection of the pairing terms on the Fermi surface(FS) using the diagonalizing matrix and scrutinize the nature of the pairings, occurring near the FS. The method is shown elaborately for RSW and Luttinger systems.

### A. Band diagonalizing of RSW Hamiltonian

The linear model for spin-3/2 RSW systems takes the form

$$\mathcal{H}_{\rm RSW}(\alpha) = v(\mathbf{J}\cdot\mathbf{k} - \alpha\mathbf{J}^3\cdot\mathbf{k}) - \mu. \tag{S1}$$

The unitary matrix $\mathcal{D}_\alpha$, diagonalizing the above $4\times 4$ Hamiltonian has the forms for $\alpha = 0$ and $4/7$

$$\mathcal{D}_{\alpha=0} = \begin{pmatrix} -e^{-3i\phi}\sin^3\left(\frac{\theta}{2}\right) & \frac{1}{2}\sqrt{3}e^{-3i\phi}\sin\left(\frac{\theta}{2}\right)\sin(\theta) & e^{-3i\phi}\cos^3\left(\frac{\theta}{2}\right) & -\frac{1}{4}\sqrt{3}e^{-3i\phi}\sin^2(\theta)\csc\left(\frac{\theta}{2}\right) \\ \frac{1}{2}\sqrt{3}e^{-2i\phi}\sin\left(\frac{\theta}{2}\right)\sin(\theta) & -\frac{1}{2}e^{-2i\phi}\sin\left(\frac{\theta}{2}\right)(3\cos(\theta)+1) & \frac{1}{4}\sqrt{3}e^{-2i\phi}\sin^2(\theta)\csc\left(\frac{\theta}{2}\right) & \frac{1}{4}e^{-2i\phi}\left(\cos\left(\frac{\theta}{2}\right)+3\cos\left(\frac{3\theta}{2}\right)\right) \\ -\frac{1}{4}\sqrt{3}e^{-i\phi}\sin^2(\theta)\csc\left(\frac{\theta}{2}\right) & \frac{1}{4}e^{-i\phi}\left(\cos\left(\frac{\theta}{2}\right)+3\cos\left(\frac{3\theta}{2}\right)\right) & \frac{1}{2}\sqrt{3}e^{-i\phi}\sin\left(\frac{\theta}{2}\right)\sin(\theta) & -\frac{1}{4}e^{-i\phi}\left(\sin\left(\frac{\theta}{2}\right)-3\sin\left(\frac{3\theta}{2}\right)\right) \\ \cos^3\left(\frac{\theta}{2}\right) & \frac{1}{4}\sqrt{3}\sin^2(\theta)\csc\left(\frac{\theta}{2}\right) & \sin^3\left(\frac{\theta}{2}\right) & \frac{1}{2}\sqrt{3}\sin\left(\frac{\theta}{2}\right)\sin(\theta) \end{pmatrix},$$

$$\mathcal{D}_{\alpha=4/7} = \begin{pmatrix} e^{i\phi}\cos\left(\frac{\theta}{2}\right) & 0 & -e^{i\phi}\sin\left(\frac{\theta}{2}\right) & 0 \\ 0 & e^{-i\phi}\sin\left(\frac{\theta}{2}\right) & 0 & -e^{-i\phi}\cos\left(\frac{\theta}{2}\right) \\ 0 & \cos\left(\frac{\theta}{2}\right) & 0 & \sin\left(\frac{\theta}{2}\right) \\ \sin\left(\frac{\theta}{2}\right) & 0 & \cos\left(\frac{\theta}{2}\right) & 0 \end{pmatrix}. \tag{S2}$$

Where, the angles $\theta$ and $\phi$ represent the direction of the $\boldsymbol{k}$-vector, i.e. $\hat{k}_x = \sin(\theta)\cos(\phi)$, $\hat{k}_y = \sin(\theta)\sin(\phi)$ and $\hat{k}_x = \cos(\theta)$. It can now be directly checked that

$$\mathcal{D}^\dagger_{\alpha=0}\mathcal{H}_{\rm RSW}(\alpha=0)\mathcal{D}_{\alpha=0} = \text{diag.}(3,1,-1,-3)v|\boldsymbol{k}|/2 - \mu,$$
$$\mathcal{D}^\dagger_{\alpha=4/7}\mathcal{H}_{\rm RSW}(\alpha=4/7)\mathcal{D}_{\alpha=4/7} = \text{diag.}(1,1,-1,-1)3v|\boldsymbol{k}|/7 - \mu. \tag{S3}$$

The first (last) two eigenvalues correspond to the conduction (valence) band. Upon isolating the effective Hamiltonian for the valence and conduction bands, they can be Nambu doubled, as shown in the main manuscript.

### B. Band diagonalizing of Luttinger Hamiltonian

The Hamiltonian for spin-3/2 Luttinger fermions displaying biquadratic band touching reads

$$\mathcal{H}_{\rm Lutt}(\mathbf{k}) = \left(\frac{\mathbf{k}^2}{2m_0} - \mu\right)\Gamma_0 - \frac{1}{2m}\sum_{a=1}^{5} d_a(\mathbf{k})\Gamma_a, \tag{S4}$$

where $\Gamma_0$ is a four-dimensional identity matrix. The $d$-vector is given by

$$d_1 = \sqrt{3}k_y k_z, \quad d_2 = \sqrt{3}k_x k_z, \quad d_3 = \sqrt{3}k_y k_x \quad d_4 = \frac{\sqrt{3}}{2}\left[k_x^2 - k_y^2\right] \quad d_5 = \frac{1}{2}\left[2k_z^2 - k_x^2 - k_y^2\right]. \tag{S5}$$

The anti-commuting $\Gamma$ matrices, which provides a basis for symmetric traceless tensors, are given by

$$\Gamma_1 = \kappa_3\sigma_2, \quad \Gamma_2 = \kappa_3\sigma_1, \quad \Gamma_3 = \kappa_2\sigma_0, \quad \Gamma_4 = \kappa_1\sigma_0, \quad \Gamma_5 = \kappa_3\sigma_3. \tag{S6}$$

Pauli matrices $\kappa$ and $\sigma$ operate on the sign and magnitude of the spin projection $m_s$, respectively. For this system, the diagonalizing matrix is given by [1]

$$\mathcal{D} = \left[2\left(1+\hat{d}_5\right)\right]^{-1/2}\left[\left(1+\hat{d}_5\right)\Gamma_0 + i\sum_{a=1}^{4}\Gamma_{a5}\right], \tag{S7}$$

where $d(\mathbf{k}) = \mathbf{k}^2\hat{d}(\mathbf{k})$ and $\Gamma_{ab} = [\Gamma_a, \Gamma_b]/(2i)$. The unitary rotation by the diagonalizing matrix leads to

$$\mathcal{D}^\dagger \mathcal{H}_{\rm Lutt}(\mathbf{k})\mathcal{D} = \left(\frac{\mathbf{k}^2}{2m_0} - \mu\right)\Gamma_0 - \frac{\mathbf{k}^2}{2m}\,\text{diag.}(1,1,-1,-1). \tag{S8}$$

The first (last) two eigenvalues correspond to the valence (conduction) band when $m_0 > m$. After isolating the effective Hamiltonian for the valence and conduction bands, they can be Nambu doubled. See the main manuscript.

### C. Band projection of local pairings

Following the Pauli exclusion principle, we are only allowed to have pairings which have a completely imaginary representation in the Dirac operator notations. Thus we can have only *six* channels for local pairings, which in a decorated Nambu spinor basis (after absorbing $\Gamma_{13}$ in the hole part of the Nambu spinor) take the form

$$\mathcal{H}^{pp}_{local} = \left[\eta_1\cos(\phi) + \eta_2\sin(\phi)\right]\sum_{d=0}^{5}\Delta_d\Gamma_d. \tag{S9}$$

Pauli matrices $\eta$ operate on the Nambu index. The $U(1)$ gauge redundancy of the global phase of the Nambu basis in (S9), we can choose $\phi = 0$ for all further calculation, without loss of generality. We project all the pairing matrices ($\hat{M}_{4\times4}$) on to the Fermi surface in conduction (or valence) band using the appropriate diagonalizing matrix

$$\mathcal{D}^\dagger\hat{M}_{4\times4}\mathcal{D} = \begin{bmatrix}\hat{a}_{2\times2} & \hat{b}_{2\times2}\\ \hat{c}_{2\times2} & \hat{d}_{2\times2}\end{bmatrix}. \tag{S10}$$

In the final expression, $\hat{a}_{2\times2}$ $\left(\hat{d}_{2\times2}\right)$ captures the form of a given pairing $\left(\hat{M}_{4\times4}\right)$ on conduction (valence) bands, while two other entries, namely, $\hat{c}_{2\times2}, \hat{b}_{2\times2}$ capture the coupling between the valence and conduction bands. Throughout this work we neglect such coupling assuming that the pairing only takes place in the close proximity to the Fermi surface, realized on the valence or conduction band.

#### 1. *Projection of local parings on Fermi surface in RSW metal*

For all forthcoming analyses, we are mostly interested in the $\alpha = 0$ case. For this value of $\alpha$, each of the valence and conduction band will have two sub-bands, which in all context of the discussion are named 3/2 and 1/2 bands. Another thing to be observed here is that, in this case the for pairing $\hat{M}_{4\times4}$ projection will have a more general form

$$\mathcal{D}^\dagger\hat{M}\mathcal{D} = \sum_{i=0}^{3} a_i\sigma_i \tag{S11}$$

near the FS. Neglecting the $a_0$ factor, as it contributes to the trivial gapped $s$-wave pairing only, we have a general form of the energies for the two bands for $\alpha = 0$ case for sub-bands $j = 3/2, 1/2$ as

$$E^0_j = \pm\left[\Delta_d^2 a_3^2 + \left(\sqrt{(vk-\mu)^2 + \Delta_d^2(a_1^2+a_2^2)} + (-1)^{j+1/2}vk/2\right)^2\right]^{1/2}. \tag{S12}$$

For $\alpha = 4/7$, with doubly degenerate valence and conduction band, the energy eigenvalues are

$$E^{4/7} = \pm\left[\left(\frac{3}{7}vk - \mu\right)^2 + \Delta_d^2(a_1^2+a_2^2+a_3^2)\right]^{1/2}. \tag{S13}$$

Nodal loops can be found from the zeros of the energies in $k$-space, which are reported in the main manuscript. All the angle-dependent functions $a_\mu \equiv a_\mu(\hat{\mathbf{k}})$ are reported in Table I of the main manuscript.

| **Pairing** | **Projection of the pairing** | **Nodal lines** |
|---|---|---|
| $\Delta_0\Gamma_0$ | $\Delta_0\sigma_0$ | $\times$ |
| $\Delta_1\Gamma_1$ | $\sqrt{3}\Delta_1(\hat{k}_y\hat{k}_z)\sigma_0$ | $k_x^2+k_y^2=k_F^2, k_y=0$<br>$k_x^2+k_y^2=k_F^2, k_z=0$ |
| $\Delta_2\Gamma_2$ | $\sqrt{3}\Delta_2(\hat{k}_x\hat{k}_z)\sigma_0$ | $k_y^2+k_z^2=k_F^2, k_x=0$<br>$k_x^2+k_y^2=k_F^2, k_z=0$ |
| $\Delta_3\Gamma_3$ | $\sqrt{3}\Delta_3(\hat{k}_x\hat{k}_y)\sigma_0$ | $k_y^2+k_z^2=k_F^2, k_x=0$<br>$k_x^2+k_z^2=k_F^2, k_y=0$ |
| $\Delta_4\Gamma_4$ | $\frac{\sqrt{3}}{2}\Delta_4(\hat{k}_x^2-\hat{k}_y^2)\sigma_0$ | $k_x^2+k_y^2+k_z^2=k_F^2, k_z=k_y$<br>$k_x^2+k_y^2+k_z^2=k_F^2, k_x=-k_y$ |
| $\Delta_5\Gamma_5$ | $\frac{1}{2}\Delta_5(2\hat{k}_z^2-\hat{k}_x^2-\hat{k}_y^2)\sigma_0$ | $\sqrt{k_x^2+k_y^2}=k_F\sqrt{2/3}, k_z=k_F/\sqrt{3}$<br>$\sqrt{k_x^2+k_y^2}=k_F\sqrt{2/3}, k_z=-k_F/\sqrt{3}$ |

Table I. The band diagonalization method executed on six local pairings for the Luttinger System. The first column presents the original form of pairing, second column represents the form after projecting the local pairings onto the FS using the diagonalization matrix and third column represent the nodal lines where the energy eigenvalues are zero.

### *2. Projection of local pairings on Fermi surface in Luttinger metal*

Now we calculate the projections of the local pairings for the Luttinger system, which will look like $\mathcal{D}^\dagger\hat{M}\mathcal{D}=a_0(\hat{\mathbf{k}})\sigma_0$. The functions $a_0(\hat{\mathbf{k}})$ are shown in Table I. The energy eigenvalues for the projected Hamiltonian are of the form

$$E_L(\mathbf{k})=\pm\sqrt{\left(\frac{k^2}{2m}-\mu\right)^2+\Delta_d^2a_0^2}. \tag{S14}$$

Taking this energy equal to zero gives us the nodal loops, also summarized in Table I.

## S2. EVOLUTION OF POLAR HAIRS AND NODAL RINGS

In this section, we are interested in the $\alpha=0$ case. We will scrutinize the impact of the pairing amplitude $\delta_d=\Delta_d/\mu$ $(d=1,2,3,4,5)$ in the structure of polar hairs and nodal rings, bringing out their unique characteristics. We find the Fermi momenta by taking $a_1=a_2=a_3=0$ in Eq. (S11), giving $k_{Fj}=\mu/jv$ and for the $j=1/2,3/2$ sub-bands.

Now, we will discuss the evolution of polar hairs over $\Delta_d$s, specifically for the pairing involving $\Delta_3$ as all the pairings $\Delta_1,\Delta_2$ and $\Delta_4$ display the evolutions, subjected to rotations about suitable axis. First, we need to observe that the magnitude of energy in Eq. (S11) is (we are interested in zeros of these energies, thus sign does not matter) lower bounded by $\Delta_d a_3$. Thus any solution for zero of the energy will require $a_3=0$ in its condition.

In case of pairing $\Delta_3$, we will have

$$a_3=\frac{\sqrt{3}}{2}\sin^2\theta\sin 2\phi=0\Rightarrow\phi=\{m\pi,(m+1/2)\pi\}\forall m\in\mathbb{Z};\ \theta\in[0,2\pi]. \tag{S15}$$

This will make $a_1=0$ and $a_2^2=\sin^2\phi$ . To progress further, it will be useful to define a set of dimensionless quantities

$$q_j=vk_j/\mu; q=vk/\mu\forall j=x,\varepsilon,z. \tag{S16}$$

Feeding all these back to the energy expression Eq. (S11) and after some calculations, we find

$$\sin^2\theta=\frac{1}{\delta_3^2}\left[q^2/4-(q-1)^2\right]=f(q)/\delta_3^2. \tag{S17}$$

We define $f(q)$ to shorten expressions. The range of $\sin\theta$ in LHS gives us domain of $q$ with real solutions

$$0\le f(q)/\delta_3^2\le 1\Rightarrow\begin{cases}q\in[2/3,2/3+\frac{2}{3}(1-\sqrt{1-3\delta_3^2})]\cup[2-\frac{2}{3}(1-\sqrt{1-3\delta_3^2}),2]\subseteq[2/3,2] & \forall\delta_3<1/\sqrt{3}=0.577\\ q\in[2/3,2]\quad\forall\delta_3\ge 0.577.\end{cases} \tag{S18}$$

As we can see, for any $\delta_3$, the domain of $q$ lies withing $[2/3, 2]$, which corresponds to $k \in [k_{F3/2}, k_{F1/2}]$. Therefore, all the polar hairs for $\delta_3$ will occupy only the space between the two sub-band FSs. However, we need to observe the domain of $q$ and $\theta$ that can be accessed by the polar hairs across different $\delta_3$s, to understand is behavior around the critical amplitude at $\delta_3 = 1/\sqrt{3} = 0.577$.

The function $f(q)$ will achieve its maximum of 1/3 at $q = 4/3$. So for $\delta_3 \geq 1/\sqrt{3} = 0.577$, we can see in (S18) $\sin^2\theta = f(q)/\delta_3^2 \in [0, 1/3\delta_3^2] \subseteq [0, 1] \forall q \in [2/3, 2]$. However, in this range of $\delta_3 > 0.577$, the upper-bound $1/3\delta_3^2$ will make some of the $\theta$s inaccessible. Hence, for $\delta_3 > 0.577$ the polar hairs gets disjoint across the equatorial plane, leaving some $\theta$s untouched in the process and forms loop connecting the north (south) poles of the two different Fermi surfaces. On the other hand, for $\delta_3 < 0.577$s, these two pairs of polar hairs exist joining the north pole and south pole of the same Fermi surfaces. At $\delta_3 = 0.577$ is the critical point where both kind of polar hairs co-exist and crosses each other at $q = 4/3$ on the equatorial plane. By north (south), we meant the $\theta = 0(\pi)$ poles of the FSs.

For the domain $\delta_3 < 0.577$, as discussed above, the polar hairs will be joining the north and south poles of the same Fermi surfaces. Another remark that can be made about the structure is that lesser the value of $\delta_3$ is, more will the polar hairs get closer to the corresponding FSs, leaving most of the $q \in [2, 2/3]$ inaccessible. This can be concluded from Eq. (S18), where we have seen that the domain of $q$ is the shell of thickness $\frac{2}{3}(1 - \sqrt{1 - 3\delta_3^2})$ extending inside the 1/2 and outside the 3/2 FS. As we decrease $\delta_3$, the domain shell will become narrower, making the polar hairs lying closer to the Fermi surfaces, as shown in Fig. 2 of main manuscript.

For pairing $\Delta_5$, a similar method yields

$$a_3 = \frac{1}{4}(3\cos\theta + 1) = 0 \Rightarrow \theta = \pm\cos^{-1}(-1/3); \phi \in [0, 2\pi]. \tag{S19}$$

Again, plugging this back into energy equation and its solutions give

$$q = q_\pm = \frac{2}{3}[2 \pm \sqrt{1 - 2\delta_5^2}]. \tag{S20}$$

The nodal loops can be constructed from the conditions in Eqs. (S19) and (S20). As evident from Eq. (S20), at $\delta_5 = 0$, there will be 4 nodal loops across different fixed $\theta$ planes. As we increase $\delta_5$, the separation between the two loops decreases and they come closer. Finally, they merg together at $\delta_5 = 1/\sqrt{2} = 0.707$. After that, the magnitudes of $q_\pm$ become imaginary, signifying absence of any nodal loop.

## S3. FREE ENERGY AND GAP EQUATIONS

In this section, we delve into the free energy and derive the gap equations from it. Subsequently, we solve for the critical temperature and pairing amplitude at $T = 0$. These two quantities as well as their ratio follow the BCS scaling at weak coupling limit ($\Delta_d/\Omega_D \ll 1$).

### A. Rotationally symmetric RSW metal ($\alpha = 0$)

For the $\alpha = 0$, we can write the free-energy as

$$F = \frac{\Delta_d^2}{2g} - 2l^3 \sum_{j\in\{3/2,1/2\}} \int \frac{d^3\mathbf{k}}{8\pi^3} k_B T \ln\cosh\left[\frac{E_j^0(\mathbf{k})}{2k_B T}\right], \tag{S21}$$

where $l$ is lattice constant, $g$ is coupling strength, $d = 1, 2, 3, 4, 5$, and throughout we set $\hbar = 1$. Now, we will define a set of dimensionless variables

$$\tilde{\Delta}_d = \Delta_d/\mu; \quad x_j = k/k_{Fj}, \quad \varepsilon_j = x_j - 1, \quad \lambda = \frac{gl^3\mu^2}{2\pi^2 v^3}, \quad \tilde{E}_j(x_j) = E_j^0(k_{Fj}x_j)/\mu, \quad f = \frac{2\pi^2 F v^3}{a^3\mu^3}, \quad t = T/\mu. \tag{S22}$$

In terms of these dimensionless variables, we can define dimensionless free energy $f$ as

$$f = \frac{\tilde{\Delta}_d^2}{2\lambda} - \sum_{j=1/2,3/2} \int \frac{d^3x_j}{8\pi^3}\frac{k_B t}{j^3} \ln\cosh\left[\frac{E_j(x_j)}{2k_B t}\right]. \tag{S23}$$

The gap equation can be sought out by finding the extrema of free energies across $\tilde{\Delta}_d^2$, by taking $\partial f/\partial\tilde{\Delta}_d^2 = 0$. Here the energy integral will be bounded by the Debye frequency $\Omega_D$. The results are captured in terms of dimensionless

Debye frequency $\omega_D = \Omega_D/\mu$. Finally, our gap equation reads

$$\lambda^{-1} = \sum_{j=1/2,3/2} \int_{-\omega_D}^{\omega_D} (\varepsilon_j+1)^2 d\varepsilon_j \int \frac{d\Omega}{4\pi} \frac{\tanh[\tilde{E}_j(\varepsilon_j+1)/2k_Bt]}{\tilde{E}_j(\varepsilon_j+1)} \left\{ a_3^2 + \left(1 + \frac{(-1)^{j+1/2}(\varepsilon_j+1)/2j}{(\frac{\varepsilon_j+1}{j}-1)^2 + \tilde{\Delta}_d^2(a_1^2+a_2^2)}\right)(a_1^2+a_2^2) \right\}. \tag{S24}$$

Now we would look into different cases to find out characteristic parameters of the system.

### 1. Critical temperature for $\alpha = 0$

At the critical temperature $T_c$ (for us, defined as $t_c = T_c/\mu$), the pairing amplitude vanishes. So, we can solve for $t_c$ from the gap equation by setting $t = t_c$ and $\tilde{\Delta}_d = 0$ in Eq. (S24). Upon separating the angular integral, we have

$$\lambda^{-1} = \int_{-\omega_D}^{\omega_D} \frac{(\varepsilon+1)^2}{j^3\varepsilon} \left(A + (-1)^{j+1/2}\frac{B(\varepsilon+1)}{2\varepsilon+(-1)^{j-1/2}}\right) \tanh\left[\frac{\varepsilon}{2k_Bt_c}\right], \tag{S25}$$

Where, $A = \int d\Omega(a_1^2+a_2^2+a_3^2)/(4\pi) = 3/5$ and $B = \int d\Omega(a_1^2+a_2^2)/(4\pi) = 2/5$ irrespective of the pairing channel. Plugging these values back into the above equation and subsequently making a weak coupling approximation ($\omega_D <<$ 1), we find the result in terms of standard trigonometric integral, yielding

$$\begin{aligned} \lambda^{-1} &= \int_{-\omega_d}^{\omega_d} d\varepsilon \frac{(\varepsilon+1)^2}{\varepsilon} \left[\frac{672}{135} + \frac{16}{135}\frac{\varepsilon+1}{2\varepsilon-1} - \frac{16}{5}\frac{\varepsilon+1}{2\varepsilon+1}\right] \tanh\frac{\varepsilon}{2k_Bt_c} \\ &= \frac{224}{135}\int_{-\omega_d}^{\omega_d} d\varepsilon \frac{\tanh\frac{\varepsilon}{2k_Bt_c}}{\varepsilon} + \mathcal{O}(\omega_D^3) = \frac{448}{135}\left[\gamma + \log\left(\frac{2\omega_D}{\pi k_B t_c}\right)\right] \quad \forall \frac{t_c}{\omega_D} << 1. \end{aligned} \tag{S26}$$

We then end up with the final form for $t_c$ as a function of $\lambda$

$$k_Bt_c = \frac{2e^\gamma}{\pi}\omega_D e^{-\frac{0.3013}{\lambda}} \simeq 1.134\omega_D e^{-\frac{0.3013}{\lambda}}. \tag{S27}$$

### 2. Pairing amplitude at T=0 for $\alpha = 0$

As $T \to 0$, $\tanh(\tilde{E}_j/2k_Bt) \to 1$. We use this in the gap equation Eq. (S24) and run a fitting analysis to find relation between $\tilde{\Delta}_d(T=0)$ and in the weakcoupling limit ($\tilde{\Delta}_d/\omega_D << 1$), leading to

$$\lambda^{-1} = \begin{cases} 3.319\left\{1.212 + \log\left(\frac{\omega_D}{\tilde{\Delta}_d}\right)\right\} & \text{for } \Delta_{1,2,3,4} \text{ pairings} \\ 3.319\left\{1.169 + \log\left(\frac{\omega_D}{\tilde{\Delta}_d}\right)\right\} & \text{for } \Delta_5 \text{ pairing.} \end{cases} \tag{S28}$$

Hence, the pairing amplitude at T=0 becomes

$$\tilde{\Delta}(T=0) = \begin{cases} 3.218\omega_D e^{-\frac{0.3013}{\lambda}} & \text{for } \Delta_{1,2,3,4} \text{ pairings} \\ 3.361\omega_D e^{-\frac{0.3013}{\lambda}} & \text{for } \Delta_5 \text{ pairing.} \end{cases} \tag{S29}$$

It follows from Eq. (S27) and Eq. (S29)) that the ratio

$$\frac{\Delta_d(T=0)}{k_BT_c} = \begin{cases} 2.964 & \text{for } \Delta_{1,2,3,4} \text{ pairings} \\ 2.838 & \text{for } \Delta_5 \text{ pairing.} \end{cases} \tag{S30}$$

Thereby, a BCS scaling is maintained between these two quantities, in weak coupling approximation.

## B. Lorentz symmetric RSW metal ($\alpha = 4/7$)

With the energy expression used in Eq. (S13), which we call here as $E^{4/7}$ and using the dimensionless variables as in Eq. (S22) (with $k_F = 7\mu/3v$), we get the gap equation of the form with an identical method like the former section

$$\lambda^{-1} = \int_{-\omega_D}^{\omega_D} d\varepsilon(\varepsilon+1)^2 \int \frac{d\Omega}{4\pi}\frac{a^2}{\tilde{E}_{4/7}(\varepsilon)} \tanh\left[\frac{\tilde{E}^{4/7}(\varepsilon)}{2k_Bt}\right]. \tag{S31}$$

The rescaled energy (as in Eq. (S22)) looks like

$$\tilde{E}^{4/7}(\varepsilon) = \sqrt{\varepsilon^2 + \tilde{\Delta}_d^2 a^2}, \tag{S32}$$

where $a = \sqrt{a_1^2 + a_2^2 + a_3^2}$. Now we will look into the critical temperature and zero temperature pairing amplitude.

### 1. *Critical temperature for $\alpha = 4/7$*

At the critical temperature and in the weak coupling limit ($\tilde{\Delta}_d/\omega_D \ll 1$), Eq. (S31) simplifies to

$$\lambda^{-1} = \int_{-\omega_D}^{\omega_D} d\varepsilon \frac{(\varepsilon+1)^2}{\varepsilon} \int \frac{d\Omega}{4\pi}\, a^2 \, \tanh\left[\frac{\varepsilon}{2k_B t}\right]. \tag{S33}$$

The integral of the angular function for the gapless (gapped) pairings becomes $\int d\Omega\, a^2/(4\pi) = 1/3$ (1). Then within the weak coupling approximation, the critical temperature is given by

$$k_B t_c = \begin{cases} \frac{2e^\gamma}{\pi}\omega_d e^{-\frac{3}{2\lambda}} \simeq 1.134\, \omega_D e^{-\frac{3}{2\lambda}} & \text{for } \Delta_{1,2,3} \text{ pairings} \\ \frac{2e^\gamma}{\pi}\omega_d e^{-\frac{1}{2\lambda}} \simeq 1.134\, \omega_D e^{-\frac{1}{2\lambda}} & \text{for } \Delta_{4,5} \text{ pairings.} \end{cases} \tag{S34}$$

### 2. *Pairing amplitude at T=0 for $\alpha = 4/7$*

At $T = 0$, following the same method for the $\alpha = 0$ case, within weak coupling limit ($\tilde{\Delta}_d/\omega_D \ll 1$) the gap equation Eq. (S31) reduce to

$$\lambda^{-1} = 2\int \frac{d\Omega}{4\pi} a^2 \left[\log \frac{\omega_D}{\tilde{\Delta}_d} - \log(a/2)\right]. \tag{S35}$$

For all the gapless (gapped) pairings, the integral of the angular function yields, $\int d\Omega\ a^2/(4\pi) = 1/3$ (1) and $\int d\Omega\ a^2\ \log(a/2)/(4\pi) = \frac{1}{3}\log(2.791)$ ($\log(0.5)$). So, finally we get

$$\tilde{\Delta}_d(T=0) = \begin{cases} 2.791\omega_d e^{-\frac{3}{2\lambda}} & \text{for } \Delta_{1,2,3} \text{ pairings} \\ 2\omega_d e^{-\frac{1}{2\lambda}} & \text{for } \Delta_{4,5} \text{ pairings.} \end{cases} \tag{S36}$$

Again, we will see a BCS scaling from Eq. (S34) and Eq. (S36), given by

$$\frac{\Delta_d(T=0)}{k_B T_c} = \begin{cases} 2.461 & \text{for gapless } \Delta_{1,2,3} \text{ pairings} \\ 1.764 & \text{for gapped } \Delta_{4,5} \text{ pairings.} \end{cases} \tag{S37}$$

[1] B. Roy, Sayed A. A. Ghorashi, M. S. Foster and A. H. Nevidomskyy, Phys. Rev. B **99**, 054505(2019).
